# Supplementary material for: Many-body effects in nonlinear optical responses of 2D layered semiconductors
Source: arXiv:1612.02714 ancillary file (2016-12-08)
Supplement: Supplementary file 1 [file SupplementaryMaterial.pdf]

# Supplemental Material for "Many-body effects in nonlinear optical responses of 2D layered semiconductors"

Grant Aivazian, Hongyi Yu, Sanfeng Wu, Jiaqiang Yan, David G. Mandrus,
David Cobden, Wang Yao, and Xiaodong Xu

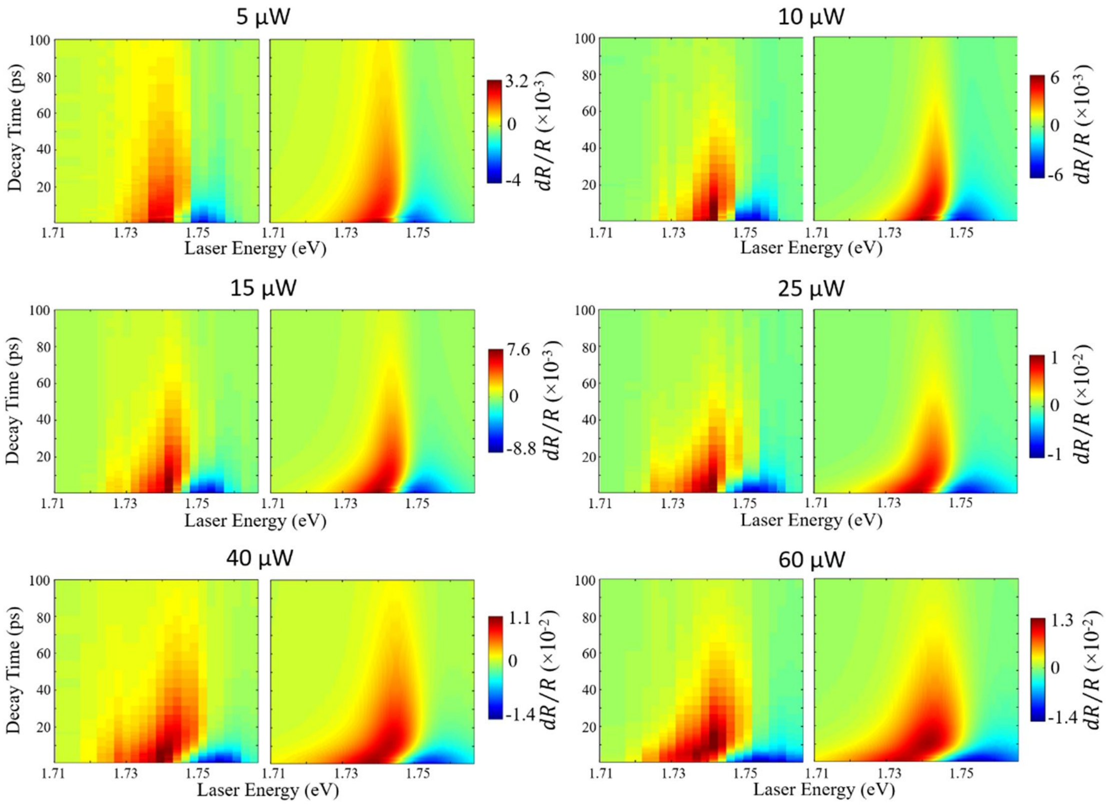


Supplementary Figure S1 | The $dR/R$ 2D map for the second sample under various pump beam power. For each power, the left figure is the measured raw data, and the right is the fit using Eq. (1) in the maintext.

## I. Exciton Optical Nonlinearities

There are various possible mechanisms of exciton optical nonlinearity. As they have been throughly discussed in early papers (see, e.g., Ref. [1] and references within), below we shall only show the results but not refer to the derivation processes.

For simplicity we shall use the well studied 2D hydrogen model. Although the excitons in monolayer TMDs exhibit nonhydrogen behaviors due to the layered geometry induced inhomogeneous dielectric constant, we expect such corrections do not change the qualitative results given below. The following parameters for monolayer TMDs will be used: $a_B \sim 1$ nm the exciton Bohr radius, $\rho_s \equiv a_B^{-2} \sim 10^{14}$ cm$^{-2}$ the exciton saturation density, $E_b \sim \frac{e^2}{\epsilon a_B} \sim 0.5$ eV the exciton binding energy. We write $\rho_X$ as the exciton density, $\rho_{\text{eh}}$ as the photo-doped free electron-hole density. Considering that the laser energy is significantly below the band-to-band transition, we expect $\rho_{\text{eh}}$ to be much smaller than the peak value of $\rho_X$.

(1) **Phase space filling**

The phase space filling effect comes from the Pauli blocking of the electrons and the holes. The interband transitions at the occupied k-space by other excitations are blocked which leads to exciton oscillator strength reduction. Following Ref. [2], the phase space filling of other excitons reduces the exciton oscillator strength to $\sim \left(1 - 7\frac{\rho_X}{\rho_s}\right)$ of that the zero density value. The phase space filling of the free carriers is also expected to scale linearly with $\rho_{\text{eh}}/\rho_s$, but as $\rho_{\text{eh}}$ is small we expect the oscillator strength reduction from the phase space filling is much smaller than that from the Coulomb screening discussed below [3].

(2) **Exciton-exciton interaction, and the estimated exciton density**

Following Ref. [2], the Coulomb interaction between two bright excitons mainly comes from the exchange of two electrons or two holes in different excitons, as illustrated in Supplementary Figure S2(a). When the two electrons or holes have the same spin and valley indices, they are indistinguishable and the exciton pairs before and after the exchange are exactly the same. This then leads to an exciton-exciton repulsive Coulomb interaction and a resonance blue shift.

When the pump frequency is near the neutral exciton resonance, the generated bright excitons can relax to the intervalley dark excitons [4] (Figure S2(b)), and also the trions (Figure S2(c)) as the sample is slightly doped. The Coulomb interactions between the bright and dark excitons and between the bright exciton and trion are analogous to that between two bright excitons, which originate from the exchange of two electrons or two holes and appear as repulsions to the bright excitons. Thus the nonlinear optical responses from the dark excitons and trions are similar to the bright excitons, which correspond to a resonance blue shift and as well as an oscillator strength reduction.

Following Ref. [2], the exciton-exciton interaction magnitude is $\Delta E_{XX} \sim 7 E_b \frac{\rho_X}{\rho_s}$ under low exciton density, which applys to the interactions between two bright excitons and between a bright and a dark exciton considering their similar wave functions. We expect

the interaction between a bright exciton and a trion to be weaker than between two bright excitons, because the trion charging energy is weaker than the exciton. For a blue shift value of $\Delta E_{+}$~0.6 meV as shown in Fig. 2(d) in the maintext, it corresponds to an exciton density $\rho_X \sim \frac{\Delta E_+}{7E_b}\rho_s \sim 10^{10}\ \mathrm{cm}^{-2}$. Considering that the discrepancy between the simplified 2D hydrogen model and the realistic non-hydrogen exciton wave function can significantly change the above $\Delta E_{XX}$ expression, this $\rho_X$ number is in reasonable agreement with the $5\times10^{11}\ \mathrm{cm}^{-2}$ value estimated from the 15 μW ($10^{13}\ \mathrm{cm}^{-2}$/pulse) pump fluence (note that the photon absorption near our monolayer $WSe_2$ exciton resonance is ~5%).

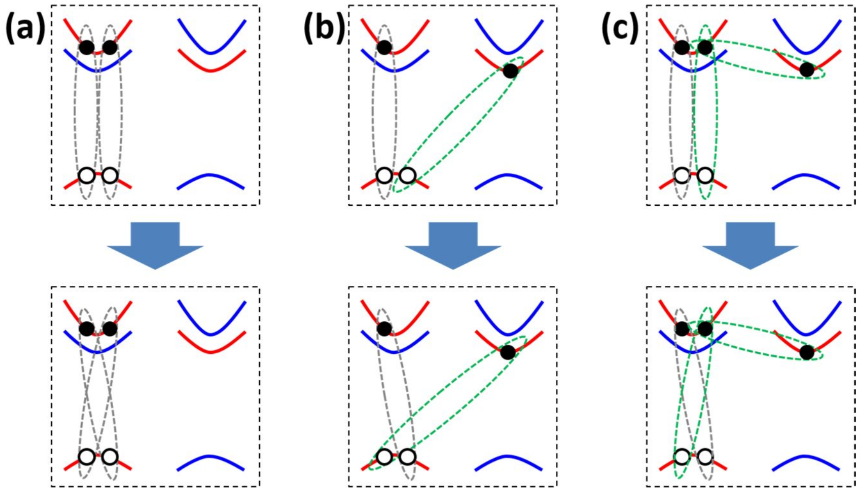


Supplementary Figure S2 | The Coulomb repulsive interactions between (a) two bright excitons, (b) a bright and a dark exciton, (c) a bright exciton and a negative trion, which originate from the exchange of two electrons or two holes in different excitons.

(3) **Band gap renormalization, and the estimated free carrier density**

The free carrier induced band gap renormalization reduces the gap value thus leads to exciton resonance red shift. The change to the gap $\Delta E_{\mathrm{g}} = -\varepsilon_X - \varepsilon_C$ includes an exchange part $\varepsilon_X$ and a correlation part $\varepsilon_C$.

The exchange part $\varepsilon_X$ is easy to calculate using Hartree-Fock approximation: $\varepsilon_X \sim \frac{e^2}{\epsilon}\sqrt{\rho_{\mathrm{eh}}} \sim E_b\sqrt{\frac{\rho_{\mathrm{eh}}}{\rho_s}}$. For $\rho_{\mathrm{eh}} \sim 10^8\ \mathrm{cm}^{-2}$, $\varepsilon_X$ can be as large as $\sim 10^{-3}E_b \sim 0.5$ meV.

For the correlation part $\varepsilon_C$ there's no simple analytical expression, while the numerical result of Ref. [5] shows $\varepsilon_C > \varepsilon_X$ under small carrier density.

For a red shift value of $\Delta E_{-}$~0.3 meV as shown in Fig. 2(d) in the maintext, it corresponds to a free carrier density $\rho_{\mathrm{eh}} \sim 10^7\ \mathrm{cm}^{-2}$ for a 15 μW pump laser.

(4) **Free carrier Coulomb screening**

Plasma screening changes the 2D Coulomb interaction to the form $V(\mathbf{k}) = \frac{2\pi e^2}{\epsilon(k+k_{\mathrm{scr}})}$ with $k_{\mathrm{scr}}$ the screening wave vector, which decreases the exciton binding energy thus leads to blue shift, and reduces the exciton oscillator strength. Under a finite tempearture T=15 K and small carrier density limit ($\rho_{\mathrm{eh}} < 10^{10}\mathrm{cm}^{-2}$), we find $k_{\mathrm{scr}} \propto \rho_{\mathrm{eh}}$ [6]. The

exciton wave function extension in **k**-space is $\sim a_B^{-1}$, so the screening induced binding energy reduction can be roughly estimated as $\Delta E_b \sim (k_{\rm scr} a_B) E_b$. For $\rho_{\rm eh} < 10^{10}$ cm$^{-2}$ we find $\Delta E_b - \varepsilon_X \lesssim 0$, thus the net effect to the exciton resonance shift is usually negative.

(5) **Oscillator strength transfer from excitons to trions**

A free charged carrier can bound with a bright exciton to form the charged exciton (trion), which is also optically active. The appearance of the trion absorption resonance is accompanied by the reduction of the exciton oscillator strength [7]. The reduction value increases linearly with $\rho_{\rm eh}$ [8]. The induced trion absorption, however, will need a nondegenerate pump-probe setup to investigate, as can be seen from the existing nondegenerate pump-probe experiments in carbon nanotubes [7] and monolayer $MoSe_2$ [9].

In our experiment we used a degenerate pump-probe setup. When the laser energy is near trion resonance (~1.715 eV), the pump excitation becomes small due to the much weaker trion absorption compared to the neutral exciton (evidenced from maintext Fig. 1b which corresponds to the linear absorption spectrum). This leads to a rather weak dR/R signal near trion resonance in maintext Fig. 1c.

(6) **Spectral broadening**

Both the excitons (including the bright, dark excitons and trions) and free carriers increase the exciton scattering rate (thus the dephasing rate), which then manifests as an increase in the resonance width $\gamma \to \gamma + \Delta\gamma$. In our model, up to the lowest order there is

$$\begin{aligned}
&\mathrm{Re}\left(\frac{1 - L(\omega)\Delta x}{\omega - E_0 + i(\gamma + \Delta\gamma)} - \frac{1}{\omega - E_0 + i\gamma}\right) \\
&\approx \mathrm{Re}\left(\frac{1 - L(\omega)(\Delta x + 2\Delta\gamma/\gamma)}{\omega - E_0 + i\gamma} - \frac{1}{\omega - E_0 + i\gamma}\right).
\end{aligned}$$

Here $L(\omega) \equiv \frac{\gamma^2}{(\omega - E_0)^2 + \gamma^2}$. We can see that the effect of $\Delta\gamma$ is similar to the oscillator strength reduction term $\Delta x$, and can be merged into $\Delta x$.

For all the nonlinear effect discussed above, only the free carrier band gap renormalization leads to the exciton resonance red shift. So we attribute the observed exciton negative energy shift (see Fig. 2(d) in the maintext) to be induced by the photo-doped free carriers. This interpretation is also consistent with the long-lived state found in monolayer $MoSe_2$ in our previous paper [10], whose signature behaviors of an opposite sign to the short component and superlinear increase with the laser power are both consistent with the free carriers. Note that in $MoSe_2$ the dark exciton has a higher energy than the bright exciton [11], thus should be not important.

For the trion, it is shown that its major part of population decays in a short time ~10 ps [12,13], comparable to the decay times of the fast components. Thus we expect that the trion nonlinear signals are mixed with those from the bright excitons, which are indistinguishable from the fast-decay components in Fig. 2c and 2d.

The lifetime of the dark exciton is expected to be longer, in principle it should result in a positive and slow-decay component to the exciton resonance shift $\Delta E$. However, in our extracted $\Delta E$ for different time delays (Fig. 2d in the maintext), we only see a fast positive and

a slow negative components. The reason that we didn't see a positive and slow component in $\Delta E$ could be that the lifetime of the dark excitons is near that of the free carriers, but the band gap renormalization effect are more pronounced so we cannot see a positive energy shift. Another explanation could be that the dark exciton has a fast nonradiative decay just like the bright exciton, e.g., captured by impuries and defects or phonon assisted Auger recombination [14]. In this case the dark exciton nonlinear signals cannot be separated from those of the bright excitons and trions because of the comparable decay time scales, and become parts of the fast component in maintext Fig. 2c and 2d.

Considering the strong Coulomb interaction effect, and the large exciton density $\rho_X$ and small free carrier density $\rho_{\mathrm{eh}}$, we expect that the many-body interaction related effects (exciton-exciton interaction, band gap renormalization, and scattering induced spectral broadening) dominate the nonlinear optical responses. The $\sqrt{\rho_{\mathrm{eh}}}$ scaling relation of $\varepsilon_X$ with the carrier density leads to a gap renormalization value $\Delta E_{\mathrm{g}}$ comparable to the exciton-exciton interaction strength $\Delta E_{XX}$, even though $\rho_{\mathrm{eh}} \ll \rho_X$ because the excitation laser energy is significantly below the band-to-band transition threshold.

## II. Effect of a large probe fluence

In our measurements, the probe beam power was set by optimizing the signal to noise ratio while keeping the integration time reasonable. Under the current probe beam power (15 μW), it took about 30 minutes to finish one delay stage scan and a 2D dR/R map shown in Fig 1c took roughly about 2 days. It approaches the tolerance limit of our setup, determined by, for example, the stability of our system. Lower probe power leads to smaller signal to noise ratio, requires longer time, and is thus not employed. Such a high probe power (15 μW, i.e., comparable to the pump fluence or even higher) could result in some probe induced nonlinear effect.

In maintext Fig. 3f, we showed the exciton resonance width $\gamma$ as a function of the pump power. In the ideal case with an infinitely weak probe pulse, we expect $\gamma$ to continuously decrease with the reduction of pump power, and ultimately approach the ~6 meV value in Fig. 1b when the pump power goes to 0. In maintext Fig. 3f we can see that, for a pump power higher than the probe power (15 μW) $\gamma$ indeed decreases when the pump power goes to lower values. But when the pump power is below the probe power, $\gamma$ keeps nearly a constant. This could be a signature of probe induced linewidth broadening.

## III. Valley coherence effect to the nonlinear optical response

The valley decoherence time in $WSe_2$ is found to be rather short (<1 ps, see [15]). Thus the valley coherence should not affect our detected signals, which focus on optical dynamics with pump-probe delay >1 ps.

Even if the valley coherence lifetime is significantly longer than 1 ps, it doesn't change our nonlinear optical susceptibility form (Eq. (1) in the maintext). In Ref. [10], we have analyzed the nonlinear optical susceptibilities for both the co-circularly and cross-linearly polarized pump-probe schemes. Their difference comes from the excitation population pulsation induced by a finite pump-probe frequency detuning. In the present frequency-

degenerate pump-probe setup, the difference between the co-circular and cross-linear schemes vanishes. Only the total population of the two valleys contributes to the nonlinear optical susceptibility which leads to Eq. (1) in the maintext, while the valley coherence has a negligible effect.


[1] H. Haug and S. Schmitt-Rink, J. Opt. Soc. Am. B 2, 1135 (1985).

[2] G. Rochat, C. Ciuti, V. Savona, C. Piermarocchi, and A. Quattropani, Phys. Rev. B 61, 13856 (2000).

[3] A. Chernikov, A. M. v. d. Zande, H. M. Hill, A. F. Rigosi, A. Velauthapillai, J. Hone, and T. F. Heinz, Phys. Rev. Lett. 115, 126802 (2015).

[4] X.-X. Zhang, Y. You, S. Y. F. Zhao, and T. F. Heinz, Phys. Rev. Lett. 115, 257403 (2015).

[5] B. Vinter, Phys. Rev. B 13, 4447 (1976).

[6] H. Yu, G.-B. Liu, P. Gong, X. Xu, and W. Yao, Nat. Commun. 5, 3876 (2014).

[7] B. Yuma *et al.*, Phys. Rev. B 87, 205412 (2013).

[8] A. Esser, R. Zimmermann, and E. Runge, phys. stat. sol. (b) 227, 317 (2001).

[9] A. Singh, G. Moody, S. Wu, Y. Wu, N. J. Ghimire, J. Yan, D. G. Mandrus, X. Xu, and X. Li, Phys. Rev. Lett. 112, 216804 (2014).

[10] J. R. Schaibley *et al.*, Phys. Rev. Lett. 114, 137402 (2015).

[11] A. Arora, K. Nogajewski, M. Molas, M. Koperskiab, and M. Potemski, Nanoscale 7, 20769 (2015).

[12] G. Wang, L. Bouet, D. Lagarde, M. Vidal, A. Balocchi, T. Amand, X. Marie, and B. Urbaszek, Phys. Rev. B 90, 075413 (2014).

[13] C. Robert *et al.*, Phys. Rev. B 93, 205423 (2016).

[14] M. Danovich, V. Zólyomi, V. I. Fal'ko, and I. L. Aleiner, 2D Mater. 3, 035011 (2016).

[15] K. Hao *et al.*, Nat. Phys. 12, 677 (2016).
